# Supplementary material for: Density Distribution in Soft Matter Crystals and Quasicrystals
Source: arXiv:2010.10191 ancillary file (2021-05-27)
Supplement: Supplementary file 1 [file SNLT_Supp_Mat_v7_final_newtitle.pdf]

# Supplementary material for “Density Distribution in Soft Matter Crystals and Quasicrystals”

P. Subramanian,<sup>1</sup> D.J. Ratliff,<sup>2,3</sup> A.M. Rucklidge,<sup>4</sup> and A.J. Archer<sup>2</sup>

<sup>1</sup>*Mathematical Institute, University of Oxford, Oxford OX2 6GG, United Kingdom*

<sup>2</sup>*Department of Mathematical Sciences and Interdisciplinary Centre for Mathematical Modelling, Loughborough University, Loughborough LE11 3TU, United Kingdom*

<sup>3</sup>*Department of Mathematics, Physics and Electrical Engineering,*

*Northumbria University, Newcastle upon Tyne NE1 8ST, United Kingdom*

<sup>4</sup>*School of Mathematics, University of Leeds, Leeds LS2 9JT, United Kingdom*

## DERIVATION OF EQ. (6) IN THE PAPER

We start from Eq. (5) in the main part of the paper, which we write again here for completeness:

$$\ln(\Lambda^3 \rho) - c^{(1)}[\rho] - \beta\mu = 0. \quad (\text{S1})$$

The one-body direct correlation function in the above is defined as the following functional derivative:

$$c^{(1)}[\rho] \equiv -\beta \frac{\delta \mathcal{F}_{\text{ex}}[\rho]}{\delta \rho(\mathbf{r})} \quad (\text{S2})$$

and similarly the pair direct correlation function is obtained after taking a further derivative [1–3]:

$$c^{(2)}(\mathbf{r}, \mathbf{r}'; \rho) \equiv -\beta \frac{\delta^2 \mathcal{F}_{\text{ex}}[\rho]}{\delta \rho(\mathbf{r}) \delta \rho(\mathbf{r}')} \quad (\text{S3})$$

As described in Refs. [1–3], one can perform a functional integration of Eq. (S3) along a linear path parameterised by  $0 \leq \lambda \leq 1$  from a reference state with density  $\rho_0$  to the final state with density  $\rho(\mathbf{r})$ , such that the density profiles of the systems along the integration path are

$$\rho_\lambda(\mathbf{r}) = \rho_0 + \lambda \Delta \rho(\mathbf{r}), \quad (\text{S4})$$

where  $\Delta \rho(\mathbf{r}) = \rho(\mathbf{r}) - \rho_0$ . This integration gives

$$c^{(1)}[\rho] = c^{(1)}[\rho_0] + \int_0^1 d\lambda \int d\mathbf{r}' \Delta \rho(\mathbf{r}') c^{(2)}(\mathbf{r}, \mathbf{r}'; \rho_\lambda). \quad (\text{S5})$$

For the chemical potential value  $\mu$  at the state point of interest, we choose  $\rho_0$  to be the uniform density value that satisfies Eq. (S1). So, from Eq. (S1) we obtain

$$\ln(\Lambda^3 \rho_0) - c^{(1)}[\rho_0] - \beta\mu = 0. \quad (\text{S6})$$

Subtracting this from Eq. (S1), we obtain

$$\ln\left(\frac{\rho}{\rho_0}\right) = c^{(1)}[\rho] - c^{(1)}[\rho_0]. \quad (\text{S7})$$

From Eqs. (S5) and (S7) we obtain

$$\ln\left(\frac{\rho}{\rho_0}\right) = \int_0^1 d\lambda \int d\mathbf{r}' \Delta \rho(\mathbf{r}') c^{(2)}(\mathbf{r}, \mathbf{r}'; \rho_\lambda), \quad (\text{S8})$$

which can easily be rearranged together with a change in the order of integration, to obtain Eq. (6) in the main paper.

Although it is highly instructive to consider this formally exact result, for practical calculations it is of little use, since determining  $c^{(2)}(\mathbf{r}, \mathbf{r}'; \rho_\lambda)$  along the path of integration is very hard. However, there are various useful approximations that can be made in this equation, which lead to several of the commonly used functionals in DFT [1–3].

## DETAILS OF IMPLEMENTATION OF SNLT

In this section we give further details of our procedure for generating and solving the truncated system of equations from the ansatz proposed in the main paper in Eq. (3), that is utilised in the accompanying MATLAB computer code. The first step is to choose the particular crystal structure as well as the order of the approximation that is to be considered. The type of crystal determines the wavevectors used in the method while the order determines the number of amplitudes one must solve for. In this illustration, we choose to explain order 2 calculations to determine a face-centred cubic (FCC) crystal, but the general approach for an arbitrary order and different choice of crystal structure follows similarly.

In section 0 of the MATLAB computer program, we first set up a 3-dimensional periodic domain and load high accuracy data for the interaction potential, e.g., GEM-4 potential. This is done within lines 1-63 of the program. The next step in the procedure is to establish the set of wavevectors used in the computation, determined by the choice of crystal structure and thus a set of principal lattice vectors (PLVs). For a FCC crystal, these are the eight vectors

$$\begin{aligned} \mathbf{b}_1 &= \frac{1}{\sqrt{3}}(1, 1, 1), & \mathbf{b}_2 &= \frac{1}{\sqrt{3}}(-1, 1, 1), \\ \mathbf{b}_3 &= \frac{1}{\sqrt{3}}(1, -1, 1), & \mathbf{b}_4 &= \frac{1}{\sqrt{3}}(1, 1, -1), \end{aligned}$$

and their negatives (with  $\mathbf{b}_{i+4} = -\mathbf{b}_i$ ). We define the PLVs as the *first shell* of wavevectors, denoted as  $\mathbf{S}_1$ , and the zeroth shell as  $\mathbf{S}_0 = \{\mathbf{0}\}$ . The  $n^{\text{th}}$  shell of vectors  $\mathbf{S}_n$  is generated recursively by adding the PLVs to

the vectors within the previous shell and removing any already appearing in previous shells:

$$\mathbf{S}_n = \{\mathbf{s}_j + \mathbf{b}_k \mid \mathbf{s}_j \in \mathbf{S}_{n-1}, \mathbf{b}_k \in \mathbf{S}_1\} \setminus \cup_{j=0}^{n-1} \mathbf{S}_j.$$

These are then grouped by their wavenumber, and the field  $\phi = \ln(\rho/\rho_0)$  is expressed as the Fourier sum involving wavevectors from shells  $\mathbf{S}_0$  to  $\mathbf{S}_n$ . For example, the sum up to and including the second shell of wavevectors for the FCC crystal is

$$\begin{aligned} \phi = & \hat{\phi}_0 + \hat{\phi}_1 \sum_{|\mathbf{k}|=1} e^{i\mathbf{k}\cdot\mathbf{r}} \\ & + \hat{\phi}_{\sqrt{4/3}} \sum_{|\mathbf{k}|=\sqrt{4/3}} e^{i\mathbf{k}\cdot\mathbf{r}} + \hat{\phi}_{\sqrt{8/3}} \sum_{|\mathbf{k}|=\sqrt{8/3}} e^{i\mathbf{k}\cdot\mathbf{r}} + \hat{\phi}_2 \sum_{|\mathbf{k}|=2} e^{i\mathbf{k}\cdot\mathbf{r}}. \end{aligned} \quad (\text{S9})$$

Each sum is over modes with the same wavenumber and in doing so we assume that modes with wavenumbers that are permutations of each other have the same amplitude (namely, the crystal has full symmetry). At higher orders, modes that have the same wavenumber without wavevector indices being permutations of each other, e.g., (1, 1, 5) and (3, 3, 3), need to be distinguished. Truncation of the sum (S9) at the  $n^{\text{th}}$  shell  $\mathbf{S}_n$ , along with the assumption of full symmetry, is what we refer to as order  $n$  strongly nonlinear theory (SNLT). This procedure is performed in the program between the lines 64-152.

With the crystal and order of the SNLT now chosen, the system of equations for SNLT are generated by projecting Eq. (9) from the main text onto one Fourier mode from each amplitude grouping illustrated in (S9). For each of these Fourier modes, with wavevector  $\mathbf{k} \neq \mathbf{0}$ , the projected equation is

$$\hat{\phi}_k + \rho_0 \beta \hat{v}(k) \int e^{\phi} e^{-i\mathbf{k}\cdot\mathbf{r}} d\mathbf{r} = 0. \quad (\text{S10})$$

where  $k = |\mathbf{k}|$  and the integral is performed over the domain of the problem. The convolution is expressed as a product in Fourier space. There is also the additional equation at zero wavenumber for the bulk mode which involves the chemical potential:

$$\hat{\phi}_0 + \rho_0 \beta \hat{v}(0) \int e^{\phi} d\mathbf{r} - \beta \mu^* = 0. \quad (\text{S11})$$

These coupled nonlinear equations for the amplitudes  $\phi_k$  are solved, for example using MATLAB's `fsolve` routine. In practice, rather than fix  $\beta\mu^*$  and solve for all the  $\hat{\phi}_k$  amplitudes, we fix  $\hat{\phi}_1$  and solve for  $\beta\mu^*$  and the other  $\hat{\phi}_k$  ( $k \neq 1$ ) amplitudes. This circumvents the need for an arclength continuation to traverse any saddle nodes that the branches may possess. As the solutions are found along each branch, we also minimize the grand potential with respect to the unit cell size, as described in [4]. This part of the procedure is performed between lines 154-374.

Other crystal structures, such as body-centred cubic (BCC) and quasicrystals (QCs), can be treated in a similar way using this procedure. To do so, one simply chooses a different set of PLVs. The field  $\phi$  in each case has an expansion analogous to (S9) but involves different wavenumbers, but again generates equations of the form (S10) and (S11) to solve.

The degrees of freedom (DOF) of the order  $n$  SNLT is the number of mode groupings, and thus amplitudes one must solve for, which changes according to the choice of lattice. This is given for some common crystal and QC structures, including BCC, FCC and IQCs, in Table I. This highlights the differences between the various different crystals, in particular the significant difference between the periodic structures and the IQC (as explained in the main paper). We observe that going to successive orders of SNLT in determining crystal density profiles leads to the addition of larger wavenumbers, e.g., orders 4 and 5 for FCC crystals only contribute at wavenumbers  $k > 2.309$ . However, for quasicrystals we observe that successive orders of SNLT can contribute to small wavenumbers. This implies that, as discussed in the main paper, there is no clear cutoff in the order of SNLT for computing QCs.

#### DETAILS OF THE CONSTRUCTION OF THE MODIFIED BEL POTENTIAL IN 3D

Here we provide some further details as to how the pair interaction potential used within the main paper may be constructed, as well as providing further information of the structures which emerge. Following Barkan et al. [5], we start with the Gaussian damped polynomial

$$v(r) = e^{-\frac{1}{2}\sigma^2 r^2} \sum_{n=0}^4 C_{2n} r^{2n}, \quad (\text{S12})$$

(i.e. the BEL potential) whose Fourier transform in three dimensions is also a Gaussian damped polynomial:

$$\begin{aligned} \hat{v}(k) &= 4\pi \int_0^\infty \frac{\sin(kr)}{kr} r^2 v(r) dr \\ &= e^{-\frac{k^2}{2\sigma^2}} \sum_{m=0}^4 D_{2m} k^{2m}. \end{aligned} \quad (\text{S13})$$

To construct a family of soft potentials with two length-scales, we impose that this function in Fourier space has two equal, negative minima at  $k = 1, q$  where the choice of  $q$  depends on the desired ratio of lengthscales. For IQCs to form, we choose  $q = 2 \cos(\frac{\pi}{5})$  to promote a ten-fold symmetry [6], and the set of conditions for  $\hat{v}(k)$  that determine  $D_{2m}$  are the following equations

$$\beta \hat{v}(1) = \beta \hat{v}(q) = -\frac{1}{\rho_0}$$

| Crystal | Order | Number of modes | DOF | wavenumbers       |
|---------|-------|-----------------|-----|-------------------|
| CH      | 1     | 1               | 2   | 1                 |
|         | 2     | 2               | 4   | 1.732, 2          |
|         | 3     | 2               | 6   | 2.646, 3          |
|         | 4     | 3               | 9   | 3.464, ..., 4     |
|         | 5     | 3               | 12  | 4.359, ..., 5     |
| SC      | 1     | 1               | 2   | 1                 |
|         | 2     | 2               | 4   | 1.414, 2          |
|         | 3     | 3               | 7   | 1.732, ..., 3     |
|         | 4     | 4               | 11  | 2.449, ..., 4     |
|         | 5     | 5               | 16  | 3, ..., 5         |
| FCC     | 1     | 1               | 2   | 1                 |
|         | 2     | 3               | 5   | 1.155, ..., 2     |
|         | 3     | 3               | 8   | 1.915, ..., 3     |
|         | 4     | 6               | 14  | 2.309, ..., 4     |
|         | 5     | 6               | 20  | 3, ..., 5         |
| BCC     | 1     | 1               | 2   | 1                 |
|         | 2     | 3               | 5   | 1.414, ..., 2     |
|         | 3     | 4               | 9   | 2.236, ..., 3     |
|         | 4     | 7               | 16  | 2.828, ..., 4     |
|         | 5     | 7               | 23  | 3.606, ..., 5     |
| CDQC    | 1     | 2               | 3   | 1, 1.618          |
|         | 2     | 9               | 12  | 0.618, ..., 3.236 |
|         | 3     | 20              | 32  | 0.382, ..., 4.854 |
|         | 4     | 44              | 76  | 0.727, ..., 6.472 |
|         | 5     | 78              | 154 | 0.236, ..., 8.090 |
| IQC     | 1     | 2               | 3   | 1, 1.618          |
|         | 2     | 13              | 16  | 0.618, ..., 3.236 |
|         | 3     | 48              | 64  | 0.382, ..., 4.854 |
|         | 4     | 119             | 183 | 0.727, ..., 6.472 |
|         | 5     | 281             | 464 | 0.236, ..., 8.090 |

TABLE I: Numbers of vectors in each shell for different crystals: 2D columnar hexagons (CH), simple cubic (SC), face-centered cubic (FCC), body-centered cubic (BCC), columnar decagonal quasicrystals (CDQCs) and for icosahedral quasicrystals (IQCs). There is an additional mode at order 0, with wavenumber zero, in each case. The number of degrees of freedom (DOF) for SNLT truncated at each order and the range of wavenumbers in each shell is also given.

and

$$\left. \frac{d\hat{v}}{dk} \right|_{k=1} = \left. \frac{d\hat{v}}{dk} \right|_{k=q} = 0,$$

which originate from requiring that the system be marginally unstable at wavenumbers  $k = 1$  and  $k = q$ , i.e. that the dispersion relation  $\omega(k) = -Dk^2[1 + \rho_0\beta\hat{v}(k)]$ , where  $D$  is the diffusion coefficient, has maxima that are at zero for these wavenumbers [7]. The precise value of  $D > 0$  is irrelevant for present purposes. However,

these equations are not alone sufficient to determine  $v(r)$  and there remain three degrees of freedom, namely  $\rho_0$ ,  $\sigma$  and one of the coefficients which one can choose to be  $C_0$  without loss of generality. There is some freedom in what values can be chosen for these, however there is a link between higher  $\sigma$  values and the favourability of QCs for systems with BEL-like interactions [8]. As such, the BEL potential we use in this work has the following parameter values:

$$\begin{aligned} \rho_0 &= 2, \quad \sigma = 0.6554, \quad D_0 = 200, \\ D_2 &= -554.47, \quad D_4 = 535.02, \\ D_6 &= -211.17, \quad D_8 = 29.02. \end{aligned} \quad (\text{S14})$$

One may then obtain the corresponding pair potential in physical space (S12) by taking the inverse Fourier transform of (S13) for the above coefficients, giving

$$\begin{aligned} C_0 &= 2.5478, \quad C_2 = -1.8160, \quad C_4 = 0.3981, \\ C_6 &= -0.266788 \times 10^{-1}, \quad C_8 = 0.6012 \times 10^{-3}. \end{aligned} \quad (\text{S15})$$

However, these are not necessary for the SNLT approach, since the calculations are done in Fourier space. Figure 1(a) displays  $v(r)$  as a function of the inter-particle distance  $r$ , demonstrating how its structure changes as the coefficient  $C_6$  is varied around the above value, which herein is denoted by  $C_6^*$ . The reason for selecting this coefficient to vary is that it affects the favourability of each of the two characteristic lengthscales in the system ( $2\pi$  and  $2\pi/q$ ) more readily than any of the others. This can be seen more clearly from Fig. 1(b), which displays the corresponding Fourier transforms,  $\hat{v}(k)$ , where there are minima at the corresponding wavenumbers  $k = 1$  and  $k = q$ , which move and even disappear as  $C_6$  is varied.

Figure 2 shows the grand potential per unit volume minus the corresponding value for the liquid state for various different crystal structures obtained using our SNLT approach for the modified BEL potential. There are solution branches corresponding to periodic crystalline structures having the unit cell size determined largely by the length scale corresponding to  $k = 1$  (no prefix) and also the length scale corresponding to  $k = q$  (prefix  $q$ ). These are calculated for fixed  $C_6 = C_6^*$  and varying chemical potential  $\beta\mu^*$ . We also display the result for the IQC phase, which for larger  $\beta\mu^*$  replaces the liquid state branch as the global minimum of the grand potential.

In Fig. 3 we display again the phase diagram for the BEL system (the same as Fig. 4 in the main paper), which shows the regions where various structures are the equilibrium phases. In this figure, we also mark 6 different state points, which are labelled  $A$ - $F$ , for which we display examples of cuts through the density profiles, which are displayed in Figs. 4-6.

In Fig. 4 we display density profiles  $\rho$  from the large lattice spacing BCC at a state point near to melting (point  $A$  in Fig. 3) and far from melting (point  $B$ ). We also display  $\ln \rho$ , which allows to see further structure in these

density profiles. We see that the density distributions around the crystal lattice sites are very clearly *not* Gaussian in form.

In Fig. 5 we display  $\rho$  and  $\ln \rho$  for the IQC phase at state points  $C$  (near to melting) and  $D$  (far from melting). As mentioned in the main paper, the SNLT approach in its current form does not adequately provide a fully converged solution for QCs, and instead the density profiles from our SNLT are used as initial conditions for a Picard iterative solution scheme to determine profiles such as those displayed in Fig. 5.

Figure 6 displays  $\rho$  and  $\ln \rho$  for the  $q$ -BCC phase at state points  $E$  (near to melting) and  $F$  (far from melting) in Fig. 3. These density profiles are rather unusual and the density peaks are again clearly not Gaussian in form. Our SNLT approach is able to easily and in a computationally efficient manner capture all of these features of the density profiles.

- 
- [1] R. Evans, “The nature of the liquid-vapour interface and other topics in the statistical mechanics of non-uniform, classical fluids,” *Adv. Phys.* **28**, 143–200 (1979).
  - [2] R. Evans, “Fundamentals of Inhomogeneous Fluids,” (Marcel Dekker, Inc., 1992).
  - [3] J.-P. Hansen and I. R. McDonald, *Theory of Simple Liquids: with Applications to Soft Matter* (Academic Press, 2013).
  - [4] A. J. Archer, D. J. Ratliff, A. M. Rucklidge, and P. Subramanian, “Deriving phase field crystal theory from dynamical density functional theory: consequences of the approximations,” *Phys. Rev. E* **100**, 022140 (2019).
  - [5] K. Barkan, M. Engel, and R. Lifshitz, “Controlled self-assembly of periodic and aperiodic cluster crystals,” *Phys. Rev. Lett.* **113**, 098304 (2014).
  - [6] P. Subramanian, A. J. Archer, E. Knobloch, and A. M. Rucklidge, “Three-dimensional icosahedral phase field quasicrystal,” *Phys. Rev. Lett.* **117**, 075501 (2016).
  - [7] A. J. Archer, A. M. Rucklidge, and E. Knobloch, “Quasicrystalline order and a crystal-liquid state in a soft-core fluid,” *Phys. Rev. Lett.* **111**, 165501 (2013).
  - [8] D. J. Ratliff, A. J. Archer, P. Subramanian, and A. M. Rucklidge, “Which wave numbers determine the thermodynamic stability of soft matter quasicrystals?” *Phys. Rev. Lett.* **123**, 148004 (2019).

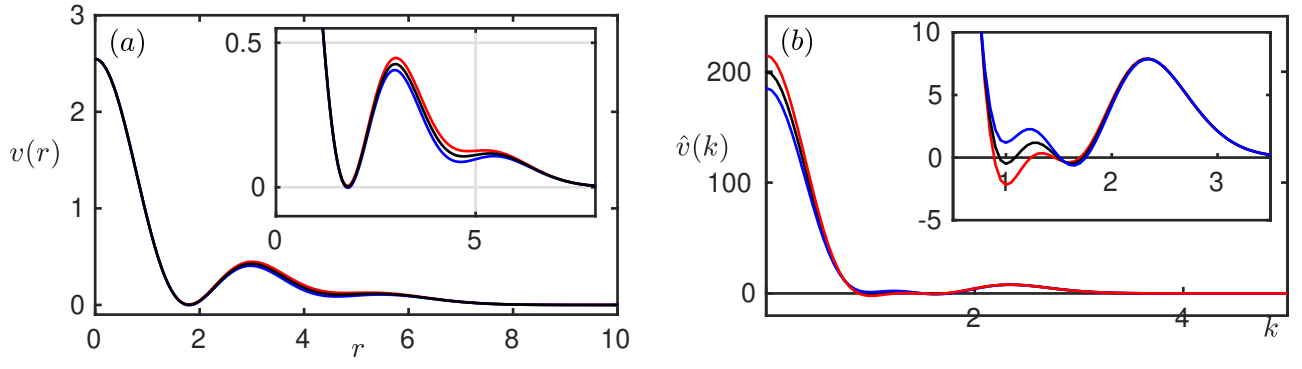

FIG. 1: Plots of the pair interaction potential in (a) physical and (b) Fourier space at the codimension 2 point (black) and at the vertical boundaries of the phase diagram, corresponding to  $C_6 - C_6^* = \pm 2 \times 10^{-4}$ , which are coloured red (plus) and blue (minus).

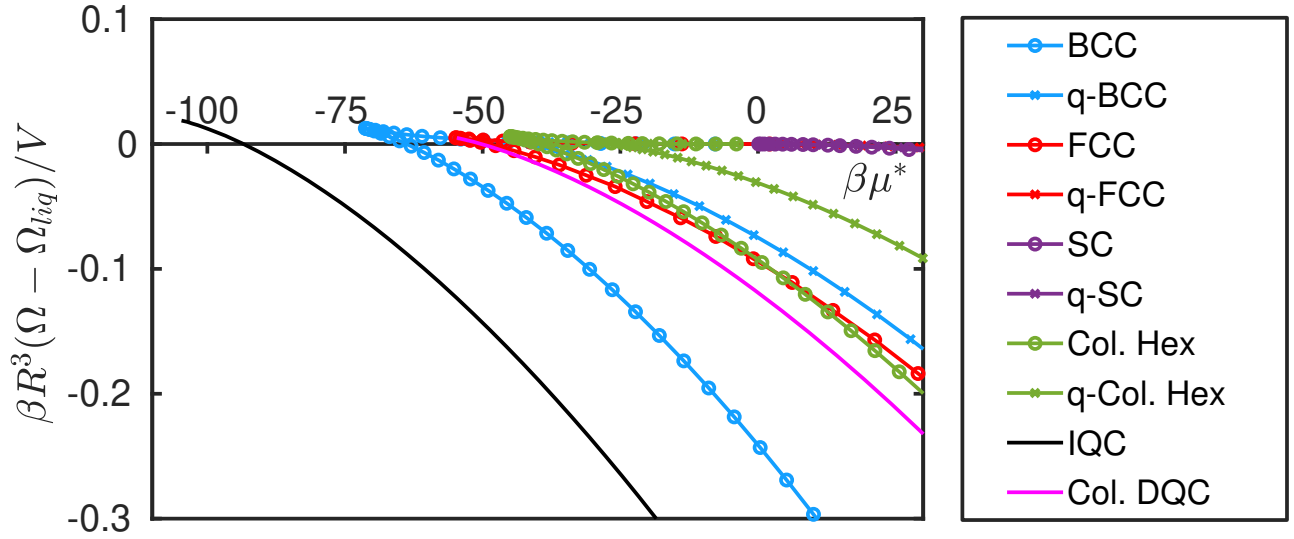

FIG. 2: A plot of  $\beta R^3(\Omega - \Omega_{liq})/V$  vs  $\beta \mu^*$  for the periodic crystals BCC, FCC, CH and SC at both lengthscales, as well as the CDQC and IQC phases obtained via Picard iteration (solid lines) emerging from this pair interaction at  $C_6 = C_6^*$ .

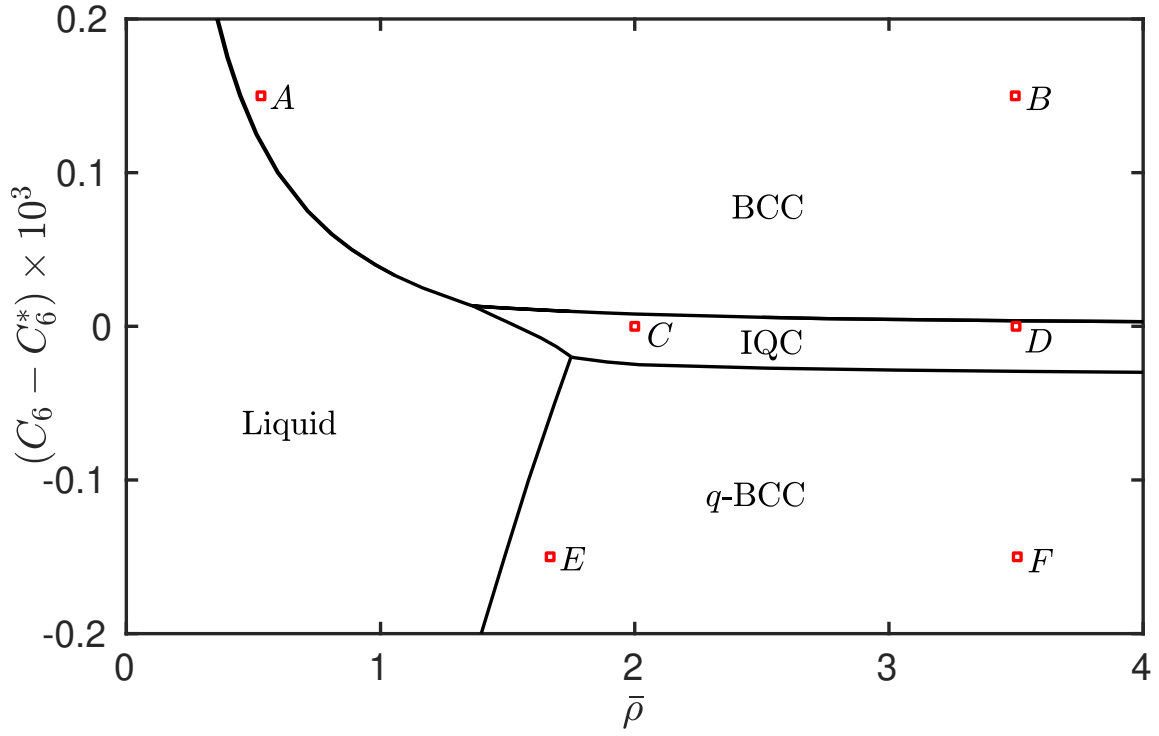

FIG. 3: The phase diagram for a system with the BEL potential (S12) with coefficients (S15) and for varying  $C_6$  and average density  $\bar{\rho}$ . The square red points labelled  $A$ - $F$  denote the state points at which the corresponding density profiles are displayed in Figs. 4–6 below.

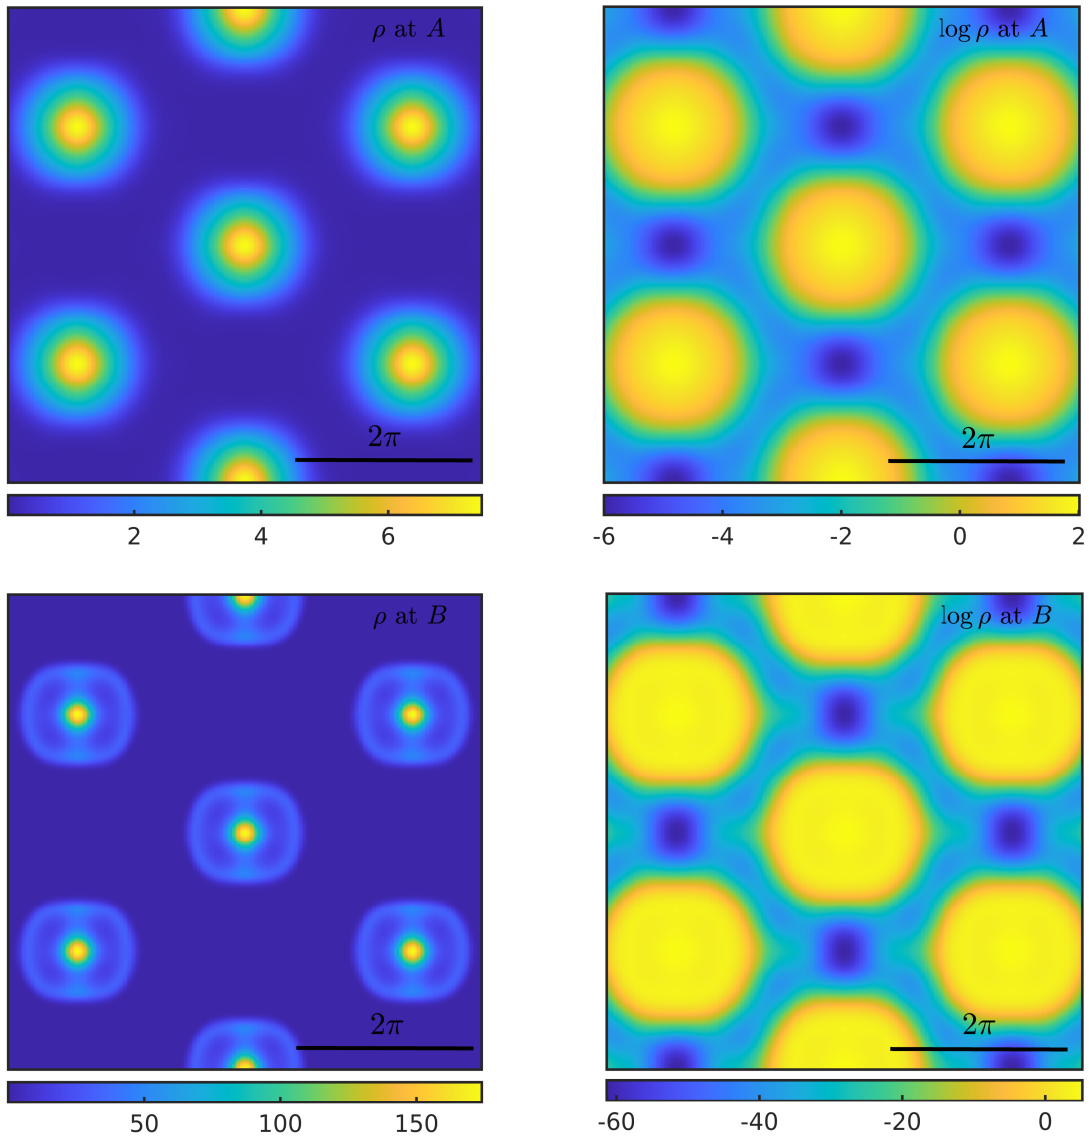

FIG. 4: The density profiles and their logarithms for the BCC crystals at state points  $A$  and  $B$  in the phase diagram Fig. 3 above. These are plotted in the plane normal to the vector  $(1, 0, 1)$ .

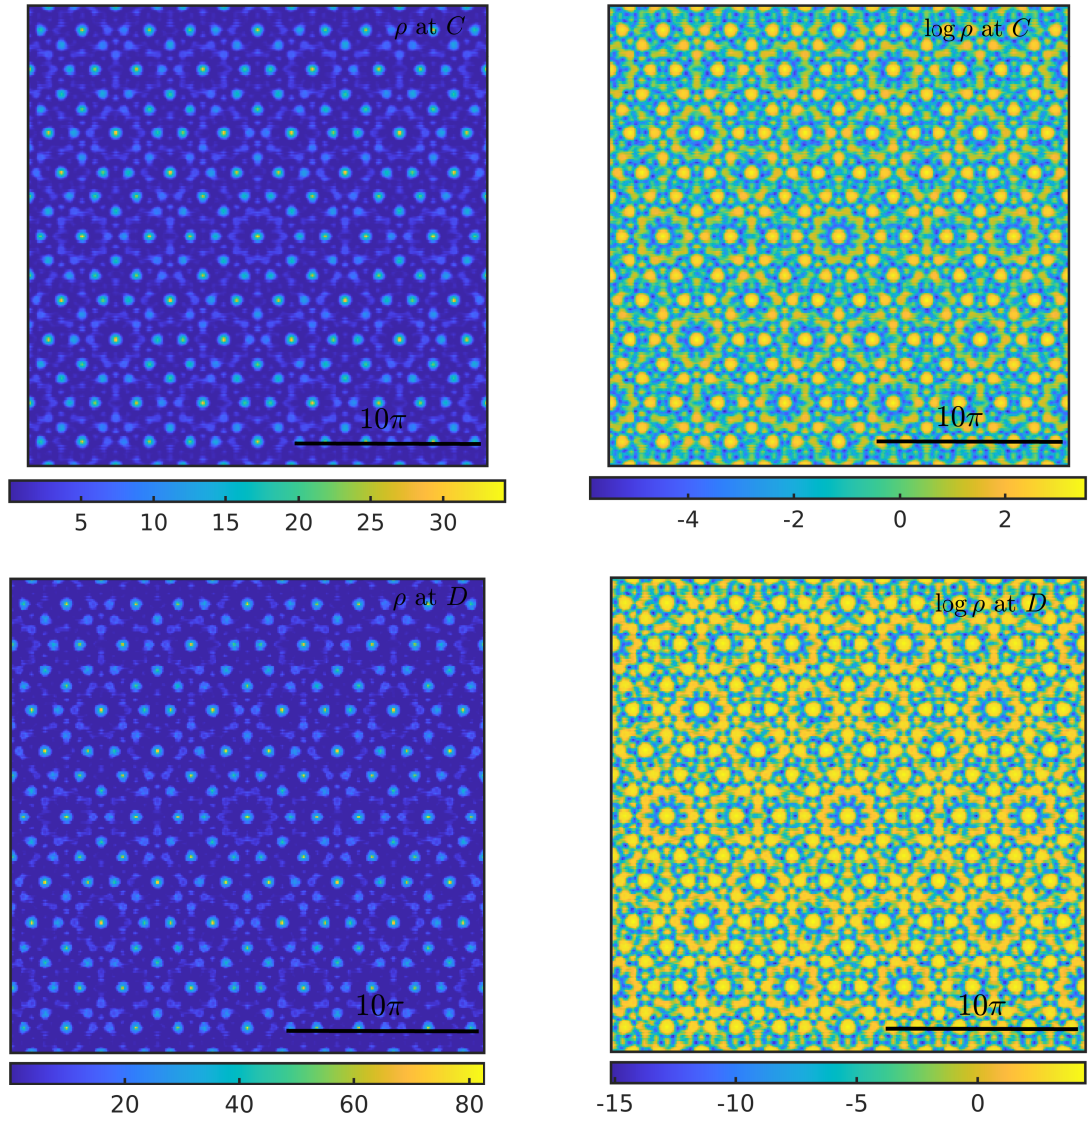

FIG. 5: The density profiles and their logarithms for the IQC phase at state points  $C$  and  $D$  in the phase diagram Fig. 3 above. These are plotted in the plane normal to the vector  $(0, -1, 2 \cos(\pi/5))$ .

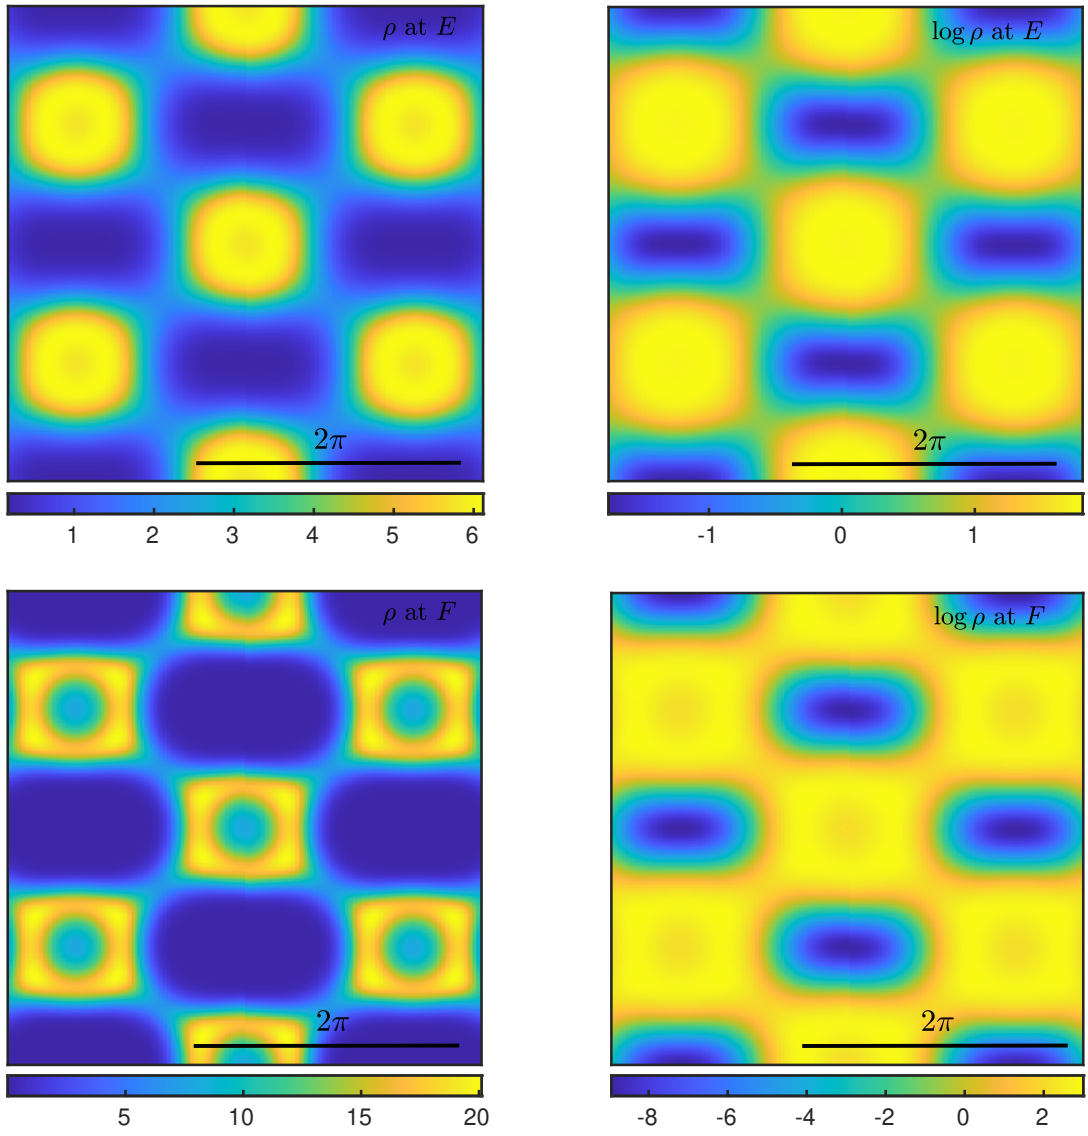

FIG. 6: The density profiles and their logarithms for the  $q$ -BCC crystals at state points  $E$  and  $F$  in the phase diagram Fig. 3 above. These are plotted in the plane normal to the vector  $(1, 0, 1)$ .
